# Supplementary material for: Delta: A Cloud-assisted Data Enrichment Framework for On-Device Continual Learning
Source: arXiv:2410.18378 source file (2024-10-24)
Supplement: Supplementary file 1 [file 8-Appendix.tex]

% \newpage
% \section{Appendix}
% \subsection{Proofs}
% \label{appendix: proofs}
